# Supplementary material for: Renormalization group approach to second-order Green's function theory
Source: arXiv:2512.11410 source file (2026-01-05)
Supplement: Supplementary file 1 [file SI.pdf]

# Renormalization group approach to second-order Green's function theory

Joshua Krieger<sup>1</sup> and Johannes Tölle<sup>2, a)</sup>

<sup>1)</sup> *University of Münster, Institute of Physical Chemistry, Corrensstraße 28/30, 48149 Münster, Germany; Center for Multiscale Theory and Computation, 48149 Münster, Germany; International Graduate School BACCARA, 48149 Münster.*

<sup>2)</sup> *Department of Chemistry, University of Hamburg, 22761 Hamburg, Germany; The Hamburg Centre for Ultrafast Imaging (CUI), Hamburg 22761, Germany; Center for Multiscale Theory and Computation, University of Münster, 48149 Münster, Germany.*

## S1. DERIVATION OF THE SRG-QSGF2 SELF-ENERGY

In this section, we present a detailed derivation of the SRG-qsGF2 self-energy given in Eq. (22) following the derivation presented in Ref. 1. Starting from the perturbative partitioning of Eq. (21), the SRG Hamiltonian and flow-generator are expanded up to second order in perturbation theory

$$\mathbf{H}(s) = \mathbf{H}^{(0)}(s, \lambda) + \lambda \mathbf{H}^{(1)}(s) + \lambda^2 \mathbf{H}^{(2)}(s). \quad (\text{S1})$$

$$\begin{aligned} \boldsymbol{\eta}(s, \lambda) &= \boldsymbol{\eta}^{(0)}(s) + \lambda \boldsymbol{\eta}^{(1)}(s) + \lambda^2 \boldsymbol{\eta}^{(2)}(s) \\ &= \left[ \mathbf{H}_d^{(0)}(s), \mathbf{H}_{\text{od}}^{(0)}(s) \right] + \lambda \left[ \mathbf{H}_d^{(0)}(s), \mathbf{H}_{\text{od}}^{(1)}(s) \right] + \lambda \left[ \mathbf{H}_d^{(1)}(s), \mathbf{H}_{\text{od}}^{(0)}(s) \right] + \lambda^2 \left[ \mathbf{H}_d^{(1)}(s), \mathbf{H}_{\text{od}}^{(1)}(s) \right] \\ &\quad + \lambda^2 \left[ \mathbf{H}_d^{(0)}(s), \mathbf{H}_{\text{od}}^{(2)}(s) \right] + \lambda^2 \left[ \mathbf{H}_d^{(2)}(s), \mathbf{H}_{\text{od}}^{(0)}(s) \right]. \end{aligned} \quad (\text{S2})$$

The flow equations for the zeroth, first and second order terms of SRG Hamiltonian can now be solved order by order. Starting at zeroth order, one finds

$$\boldsymbol{\eta}^{(0)}(s) = 0, \quad (\text{S3})$$

since  $\mathbf{H}^{(0)}(s) = \mathbf{H}^{(0)}(0) = \mathbf{H}_d$ .

Continuing with the first order Hamiltonian  $\mathbf{H}^{(1)}(s)$ , only the first term of  $\boldsymbol{\eta}^{(1)}(s)$  in Eq. S2 in combination with  $\mathbf{H}_d^{(0)}$  is non-zero.  $\mathbf{H}^{(1)}(s)$  is determined from

$$\begin{aligned} \frac{d\mathbf{H}^{(1)}(s)}{ds} &= \left[ \left[ \mathbf{H}_d^{(0)}, \mathbf{H}_{\text{od}}^{(1)}(s) \right], \mathbf{H}_d^{(0)} \right] \\ &= 2 \begin{pmatrix} \mathbf{0} & \mathbf{F}\mathbf{W}^{(1)}(s)\mathbf{C} \\ \mathbf{C}\mathbf{W}^{(1),\dagger}(s)\mathbf{F} & \mathbf{0} \end{pmatrix} - \begin{pmatrix} \mathbf{0} & \mathbf{W}^{(1)}(s)\mathbf{C}\mathbf{C} \\ \mathbf{F}\mathbf{F}\mathbf{W}^{(1),\dagger}(s) & \mathbf{0} \end{pmatrix} - \begin{pmatrix} \mathbf{0} & \mathbf{F}\mathbf{F}\mathbf{W}^{(1)}(s) \\ \mathbf{W}^{(1),\dagger}(s)\mathbf{C}\mathbf{C} & \mathbf{0} \end{pmatrix}. \end{aligned} \quad (\text{S4})$$

Considering the initial condition  $\mathbf{H}_d^{(1)}(0) = \mathbf{0}$ , it becomes clear, that  $\mathbf{H}_d^{(1)}(s) = \mathbf{0}$ , while the elements of  $\mathbf{W}^{(1)}(s)$  are given as (assuming  $F_{pq} = \delta_{pq}\epsilon_p$ )

$$\frac{dW_{p,rtu}^{(1)}(s)}{ds} = -(\epsilon_p - C_{rtu})^2 W_{p,rtu}^{(1)}(s). \quad (\text{S5})$$

Solving Eq. (S5), the elements of  $\mathbf{H}_{\text{od}}^{(1)}(s)$  become

$$W_{p,rtu}^{(1)}(s) = W_{p,rtu} e^{-s(\Delta_{tu}^{pr})^2} = \frac{1}{\sqrt{2}} \langle pr || tu \rangle e^{-s(\Delta_{tu}^{pr})^2}, \quad (\text{S6})$$

with

$$\Delta_{rs\dots}^{pq\dots} = \epsilon_p + \epsilon_q + \dots - \epsilon_r - \epsilon_s - \dots \quad (\text{S7})$$

For the The second order flow equations the evaluation of the commutators shows, that only  $\left[ \left[ \mathbf{H}_d^{(0)}, \mathbf{H}_{\text{od}}^{(2)} \right], \mathbf{H}_d^{(0)} \right]$  and  $\left[ \left[ \mathbf{H}_d^{(0)}, \mathbf{H}_{\text{od}}^{(1)} \right], \mathbf{H}_{\text{od}}^{(1)} \right]$  yield non-vanishing terms. Collecting the terms for  $\mathbf{F}^{(2)}(s)$  yields

$$\frac{dF_{pq}^{(2)}(s)}{ds} = \sum_{rtu} (\epsilon_p + \epsilon_q - 2C_{rtu}) W_{p,rtu} W_{q,rtu}^\dagger e^{-s[(\epsilon_p - C_{rtu})^2 + (\epsilon_q - C_{rtu})^2]}. \quad (\text{S8})$$

---

<sup>a)</sup> Electronic mail: jojotoel@gmail.com

Solving this equation by making use of the initial condition  $\mathbf{F}^{(2)}(s) = 0$  results in

$$F_{pq}^{(2)}(s) = \sum_{rtu} \frac{\Delta_{tu}^{pr} + \Delta_{tu}^{qr}}{(\Delta_{tu}^{pr})^2 + (\Delta_{tu}^{qr})^2} W_{p,rtu} W_{q,rtu} \left[ 1 - e^{-s[(\Delta_{tu}^{pr})^2 + (\Delta_{tu}^{qr})^2]} \right]. \quad (\text{S9})$$

By separately summing over the  $2p1h$  and  $2h1p$  parts of Eq. (S9), one obtains the second order static Fock matrix contribution  $[F_{pq}^{\text{SRG-qSGF2}}(s)]$

$$\begin{aligned} F_{pq}^{\text{SRG-qSGF2}}(s) = & \frac{1}{2} \sum_{ija} \frac{\Delta_{ij}^{pa} + \Delta_{ij}^{qa}}{(\Delta_{ij}^{pa})^2 + (\Delta_{ij}^{qa})^2} \times \langle pa || ij \rangle \langle ij || qa \rangle \times \left[ 1 - e^{-s[(\Delta_{ij}^{pa})^2 + (\Delta_{ij}^{qa})^2]} \right] \\ & + \frac{1}{2} \sum_{abi} \frac{\Delta_{ab}^{pi} + \Delta_{ab}^{qi}}{(\Delta_{ab}^{pi})^2 + (\Delta_{ab}^{qi})^2} \times \langle pi || ab \rangle \langle ab || qi \rangle \times \left[ 1 - e^{-s[(\Delta_{ab}^{pi})^2 + (\Delta_{ab}^{qi})^2]} \right]. \end{aligned} \quad (\text{S10})$$

## S2. DERIVATION OF THE SECOND-ORDER SRG-QSGF2-PT2 ENERGY CORRECTION

In this section, we present a derivation of the QP-PT2 energy correction relying on the derivation of Ref. 2 of regularized second-order perturbation theory. Making use of the Hamiltonian partitioning of Eq. (30) in the manuscript, the zeroth order flow generator  $\hat{\eta}^{(0)}(s)$  is given as

$$\hat{\eta}^{(0)}(s) = [\tilde{f}^{(0)}(s), \hat{V}^{(0)}(s)] = 0, \quad (\text{S11})$$

since  $\hat{V}^{(0)}(s) = 0$ , resulting in an  $s$ -independent zeroth order Hamiltonian  $\hat{H}^{(0)}(s) = \hat{H}^{(0)}(0)$ .

The first order flow generator is given as

$$\hat{\eta}^{(1)}(s) = [\tilde{f}^{(0)}(s), \hat{V}^{(1)}(s)] + [\tilde{f}^{(1)}(s), \hat{V}^{(0)}(s)] = [\tilde{f}^{(0)}(s), \hat{V}^{(1)}(s)], \quad (\text{S12})$$

and the first-order flow equation reads

$$\frac{d}{ds} \hat{H}^{(1)}(s) = [\hat{\eta}^{(1)}(s), \hat{H}^{(0)}(s)]. \quad (\text{S13})$$

With this, the first and second-order energy expressions become

$$\frac{d}{ds} E^{(1)} = \langle \Phi | [\hat{\eta}_1^{(1)}(s), \hat{H}_1^{(0)}] | \Phi \rangle + \langle \Phi | [\hat{\eta}_2^{(1)}(s), \hat{H}_2^{(0)}] | \Phi \rangle = 0, \quad (\text{S14})$$

and

$$\frac{d}{ds} E^{(2)}(s) = \langle \Phi | [\hat{\eta}^{(1)}(s), \hat{H}^{(1)}(s)] | \Phi \rangle, \quad (\text{S15})$$

where  $\hat{\eta}_1$ ,  $\hat{\eta}_2$ ,  $\hat{H}_1$  and  $\hat{H}_2$  denote the one- and two-body parts of  $\hat{\eta}$  and  $\hat{H}$ , respectively. Eq. S15 can be decomposed into its one- and two-body contributions

$$\frac{d}{ds} E_1^{(2)}(s) = \langle \Phi | [\hat{\eta}_1^{(1)}(s), \hat{H}_1^{(1)}(s)] | \Phi \rangle, \quad (\text{S16})$$

and

$$\frac{d}{ds} E_2^{(2)}(s) = \langle \Phi | [\hat{\eta}_2^{(1)}(s), \hat{H}_2^{(1)}(s)] | \Phi \rangle. \quad (\text{S17})$$

After integration and evaluation of the commutators (see for example the appendix of Ref. 2), one finds that the one-body contribution vanishes, while the two-body contribution evaluates to

$$E^{(2)}(s) = \sum_{ia} \frac{|F_{ia}^{\text{SRG-qSGF2}}|^2}{\text{QP} \Delta_a^i} \left[ 1 - e^{-2s(\text{QP} \Delta_a^i)^2} \right] + \frac{1}{4} \sum_{ijab} \frac{|\langle ij || ab \rangle|^2}{\text{QP} \Delta_{ab}^{ij}} \left[ 1 - e^{-2s(\text{QP} \Delta_{ab}^{ij})^2} \right]. \quad (\text{S18})$$

## S3. RI-QSGF2 WITH THE NATURAL AUXILIARY FUNCTIONS APPROXIMATION

The natural auxiliary functions (NAF) approximation<sup>3,4</sup> removes redundant information within the auxiliary basis through transformation of the resolution of the identity (RI) integral tensor<sup>5,6</sup> in a compressed auxiliary function space. We refer to Ref. 7 for a more detailed description of the NAF procedure, and its implementation in molecular orbital basis in SERENITY.

Since the qsGF2 calculations of this work start from an already converged mean-field self-consistent (SCF) field solution, we investigate the option to keep the NAF matrix between SCF iterations in the qsGF2 procedure for increased computational efficiency. Table S1 contains the mean absolute differences (MADs) of the QP(SCS)-PT2 energies for different NAF thresholds compared to QP(SCS)-PT2 energies without the NAF approximation for the GW50 benchmark set.

Truncation thresholds of  $10^{-4}$  and  $10^{-3}$  result in mean reductions of the size the auxiliary basis of 12 % and 26 % respectively, while the MAD within this approximation is on the order of  $10^{-8}$  a.u. and  $10^{-7}$  a.u.. For a threshold of  $10^{-2}$ , the MAD increases to  $3.08 \cdot 10^{-6}$  a.u., while the size of the auxiliary basis set is almost halved. For a threshold of  $10^{-1}$ , the MAD increases to  $10^{-4}$  a.u., while less than a third of the auxiliary basis functions are retained. We choose a threshold of  $10^{-2}$ , since the error introduced by the NAF approximation in this case is comparable to the error already introduced by the RI approximation itself ( $0.23 \mu\text{Ha}/\text{atom}^8$  for aug-cc-pVTZ<sup>9-12</sup>). As the error introduced

TABLE S1: Mean absolute differences (MADs) in a.u. of the QP-(SCS)-PT2 energies of the GW50 benchmark set and mean ratio of retained auxiliary basis functions relative to the original auxiliary basis size mean  $n_{\text{aux}}^{\text{NAF}}/n_{\text{aux}}$  for different NAF thresholds. The NAFs were either recomputed for every SCF cycle or kept between cycles. Reference energies are QP(SCS)-PT2 without employing the NAF approximation [aug-cc-pVTZ<sup>9-12</sup>].

|                                                   | NAF threshold       |                     |                      |                      |
|---------------------------------------------------|---------------------|---------------------|----------------------|----------------------|
|                                                   | $10^{-4}$           | $10^{-3}$           | $10^{-2}$            | $10^{-1}$            |
| recompute NAFs                                    | $2.1 \cdot 10^{-8}$ | $1.6 \cdot 10^{-7}$ | $3.08 \cdot 10^{-6}$ | $1.08 \cdot 10^{-4}$ |
| keep NAFs                                         | $2.5 \cdot 10^{-8}$ | $2.8 \cdot 10^{-7}$ | $5.47 \cdot 10^{-6}$ | $1.09 \cdot 10^{-4}$ |
| mean $n_{\text{aux}}^{\text{NAF}}/n_{\text{aux}}$ | 0.88                | 0.74                | 0.56                 | 0.30                 |

by keeping the NAFs between SCF cycles is only marginally larger than recomputing them in each cycle, we keep the NAFs between iterations.

However, this results in a qsGF2 solution that is no longer strictly starting point independent, which will be investigated in the following. Figure S1 shows the mean absolute differences in the QP(SCS)-PT2 energies for the GW50 benchmark set using HF, PBE<sup>13</sup>, and PBE0<sup>13,14</sup> initial mean-field starting points. In Figure S1, the starting

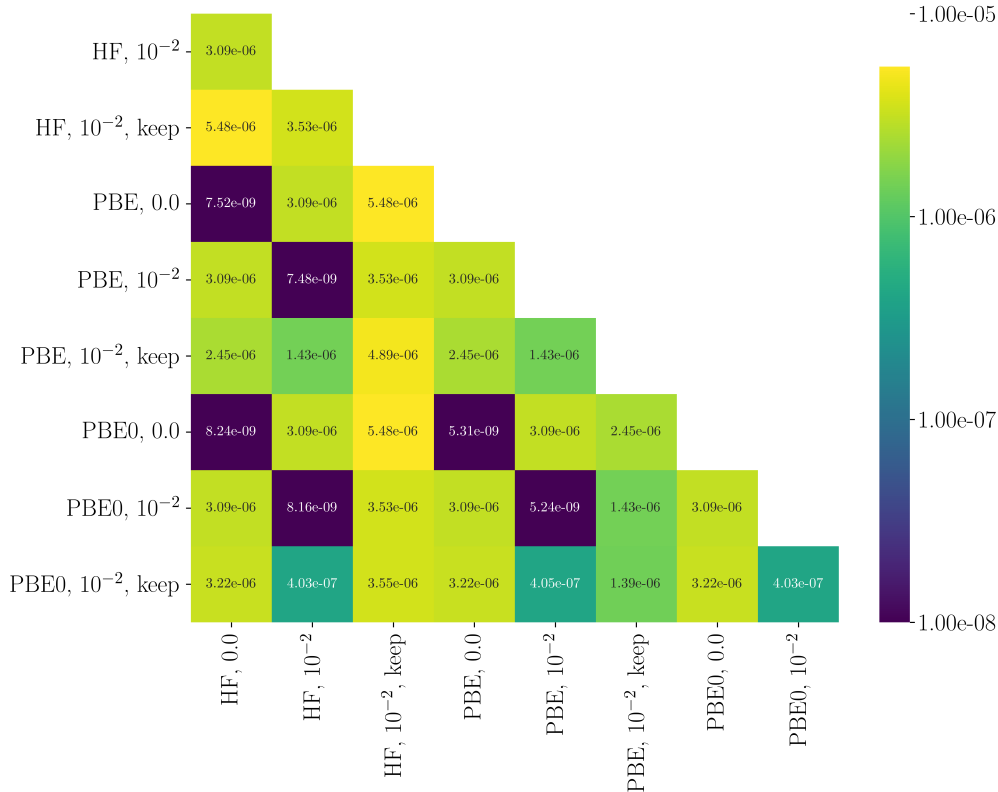

FIG. S1: Mean absolute differences (MADs) in the QP(SCS)-PT2 energies (in a.u.) for the GW50 benchmark set between HF, PBE and PBE0 mean-field starting points without the NAF approximation (denoted as 0.0), recomputing the NAFs (threshold of  $10^{-2}$ ) each SCF iteration and keeping the NAFs between iterations (denoted as keep) [aug-cc-pVTZ<sup>9-12</sup>].

point independence of qsGF2 is confirmed (without the NAF approximation and with the NAFs when recomputed at every cycle), resulting in MADs within the convergence threshold of the SCF procedure itself ( $5 \times 10^{-8}$  a.u.). When keeping the NAFs between SCF cycles, the differences between the starting points increase to the order of

$10^{-6}$  a.u., which is on the same order of magnitude as the error introduced by using the NAF approximation. We therefore conclude that the starting point dependence introduced by not recomputing the NAFs between SCF cycles is negligible.

## S4. QUASIPARTICLE ENERGIES

### A. $s$ dependence

Figure S2 depicts the IP errors with respect to  $\Delta\text{CCSD(T)}$  for the SRG-qsGF2 method as a function of  $s$  for three exemplary systems. It can be seen that no convergence with respect to  $s$  is observed for MgO.

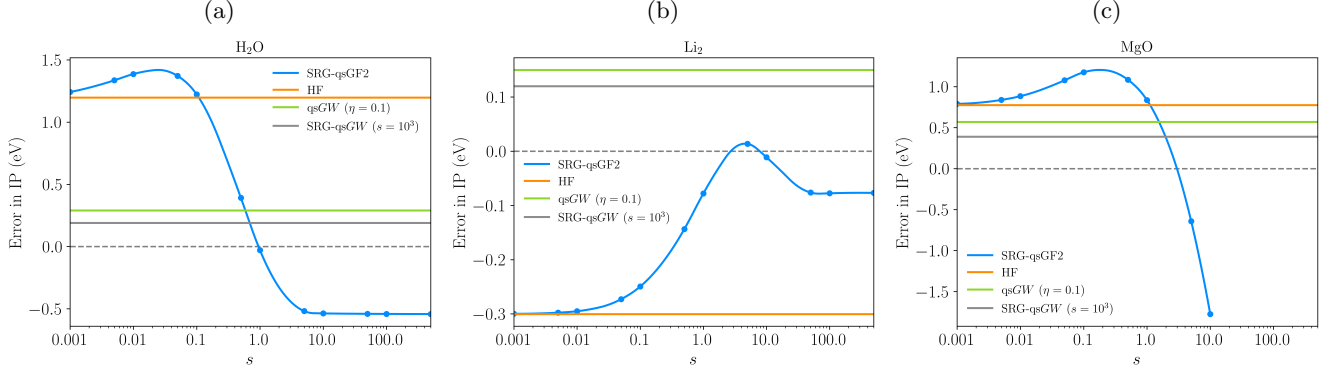

FIG. S2: Error of the IP of  $\text{H}_2\text{O}$  (a),  $\text{Li}_2$  (b) and  $\text{MgO}$  (c) with respect to  $\Delta\text{CCSD(T)}$  as a function of the SRG parameter  $s$ . The calculations for  $\text{MgO}$  didn't converge for  $s \geq 50$ . The calculations were performed using the aug-cc-pVTZ basis set<sup>9–12</sup> and the RI approximation. HF (orange), qsGW ( $\eta = 0.1$ ) (green) and SRG-qsGW<sup>1</sup> results are also shown for comparison.

### B. Parameter Optimization

Fig. S3 a) depicts the dependence of the MAE for ionization potentials (IPs) and electron affinities (EAs) as a function of the  $s$  parameter for SRG-qsGF2 for the GW50 benchmark set. It can be seen that the MAE for the EAs shows a significantly weaker  $s$  dependence compared to the IPs. For the IPs, the smallest MAE is found for  $s = 0.525$ . Figures S3 b), c) and e) depict the dependence of the MAE for IPs/EAs depending on  $s$ , and the spin-scaling parameters  $c_{\text{OS}}/c_{\text{SS}}$ . All combinations considered in this work are shown in Figure S3 e). Again, a weaker dependence of the MAE for the EAs is observed. Slices for the spin-scaling parameters for the optimal  $s$  value are shown in Figures S3 b), c).

In the case of SRG-SOS-qsGF2 ( $s = 1.4$ ), a minimum MAE for the IPs for  $c_{\text{OS}} = 1.0$  is found. Similarly, Figures S3 d) and f) show the parameter dependence for the combined MAEs, as defined in Eq. (36) of the manuscript, for SRG-SCS-qsGF2. In this case, the optimal parameters are  $c_{\text{SS}} = 0.6$ ,  $c_{\text{OS}} = 1.0$  and  $s = 0.7$ .

The MAE, mean signed error (MSE), root mean square deviation (RMSD), standard deviation of the errors (SDE), as well as the largest errors for the parametrized SRG-qsGF2 procedures and a comparison to SRG-qsGW are shown in Table S2.

TABLE S2: Metrics of the principal IP and EA errors (in eV) for the GW50 benchmark set for SRG-sqGF2, SRG-SOS-qsGF2 and SRG-SCS-qsGF2, and the SRG-qsGW procedure<sup>1</sup>. Calculations were performed using the aug-cc-pVTZ basis set<sup>9–12</sup>, the values for the SRG-qsGW method were taken from Ref. 1.

|        | SRG-qsGF2 |       | SRG-SOS-qsGF2 |       | SRG-SCS-qsGF2 |       | SRG-qsGW |       |
|--------|-----------|-------|---------------|-------|---------------|-------|----------|-------|
| metric | IP        | EA    | IP            | EA    | IP            | EA    | IP       | EA    |
| MSE    | 0.08      | -0.04 | 0.03          | -0.17 | 0.05          | -0.09 | 0.17     | 0.04  |
| MAE    | 0.25      | 0.20  | 0.14          | 0.27  | 0.21          | 0.20  | 0.19     | 0.12  |
| RMSD   | 0.34      | 0.31  | 0.20          | 0.37  | 0.29          | 0.31  | 0.23     | 0.22  |
| SDE    | 0.33      | 0.31  | 0.19          | 0.33  | 0.28          | 0.30  | 0.16     | 0.22  |
| Min    | -1.00     | -1.00 | -0.29         | -1.26 | -0.74         | -1.10 | -0.32    | -0.25 |
| Max    | 0.78      | 1.12  | 0.65          | 1.09  | 0.75          | 1.11  | 0.42     | 1.16  |

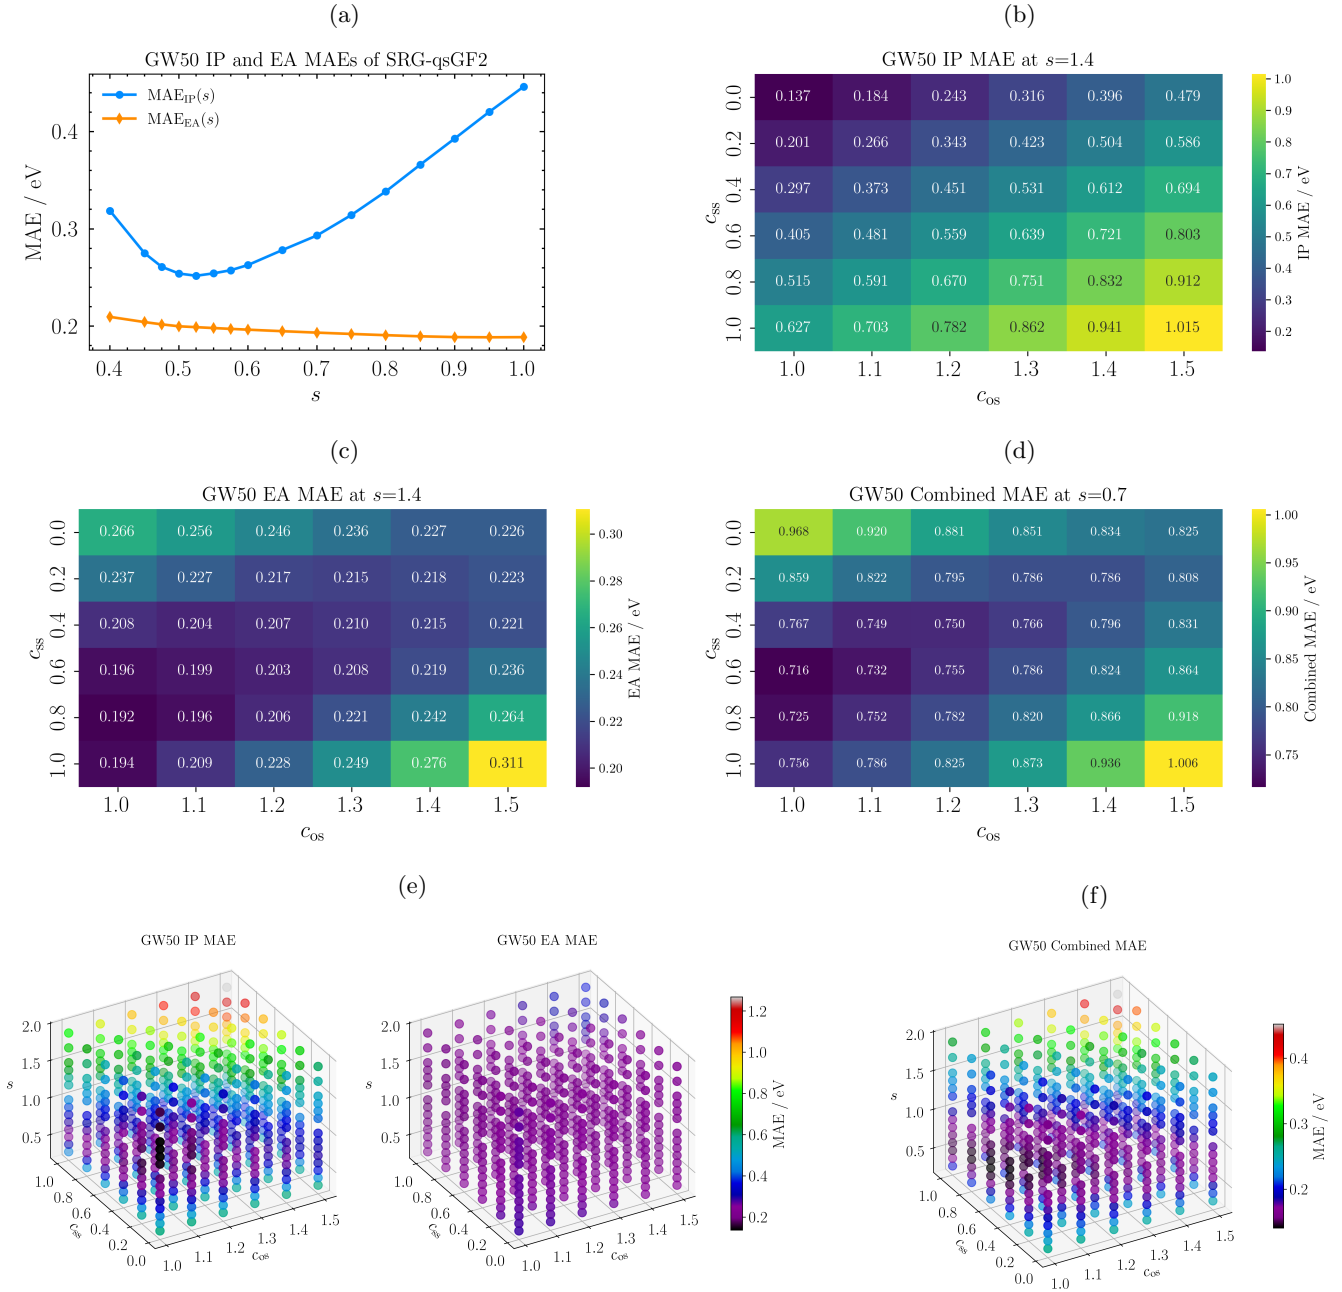

FIG. S3: MAEs and weighted MAEs [Eq. (36) in manuscript] for IPs and EAs for the GW50 benchmark set<sup>1</sup> for SRG-qsGF2: a)  $s$ -dependence; b), c)  $c_{\text{ss}}$  and  $c_{\text{os}}$  dependence for  $s = 1.4$ ; d) Weighted MAE for  $c_{\text{ss}}$  and  $c_{\text{os}}$  at  $s = 0.7$ ; e) MAE and f) weighted MAE for the investigated  $s$ ,  $c_{\text{ss}}$ , and  $c_{\text{os}}$  parameter space. Calculations were performed using the aug-cc-pVTZ basis set.<sup>9–12</sup>

# S5. DIPOLE MOMENTS

TABLE S3: Dipole Moments calculated with the methods discussed in Section IV B for the set of 37 molecules with non-zero dipole moments presented in Ref. 15. All calculations were performed using the cc-pVTZ basis set<sup>9–12</sup> and corresponding auxiliary basis set.

| system                        | SRG-<br>qsGF2 | SRG-SCS-<br>qsGF2 | SRG-SOS-<br>qsGF2 | OO-MP2 | exp. <sup>a</sup> | LR-CCSD <sup>a</sup> | MP2   | MP2 <sup>a</sup> |
|-------------------------------|---------------|-------------------|-------------------|--------|-------------------|----------------------|-------|------------------|
| Acetaldehyde                  | 2.686         | 2.688             | 2.717             | 2.580  | 2.750             | 2.834                | 2.626 | 2.625            |
| Acetic Acid                   | 1.596         | 1.597             | 1.608             | 1.541  | 1.700             | 1.709                | 1.550 | 1.550            |
| Acetone                       | 2.847         | 2.843             | 2.862             | 2.749  | 2.880             | 3.014                | 2.782 | 2.782            |
| Acetonitrile                  | 3.943         | 3.910             | 3.876             | 3.799  | 3.920             | 3.948                | 3.826 | 3.826            |
| C <sub>3</sub> H <sub>8</sub> | 0.074         | 0.075             | 0.076             | 0.081  | 0.084             | 0.085                | 0.081 | 0.081            |
| CH <sub>3</sub> F             | 1.767         | 1.785             | 1.832             | 1.783  | 1.858             | 1.889                | 1.808 | 1.805            |
| Chlorobenzene                 | 1.680         | 1.681             | 1.705             | 1.643  | 1.690             | 1.718                | 1.677 | 1.680            |
| CO                            | 0.247         | 0.223             | 0.153             | 0.313  | 0.110             | 0.106                | 0.294 | 0.294            |
| Cytosine                      | 6.343         | 6.356             | 6.412             | 6.212  | 7.000             | 6.501                | 6.311 | 6.171            |
| Dimethylamine                 | 1.026         | 1.025             | 1.035             | 0.989  | 1.010             | 1.084                | 1.011 | 1.010            |
| Dimethyl Ether                | 1.276         | 1.280             | 1.311             | 1.242  | 1.300             | 1.356                | 1.279 | 1.277            |
| Dimethyl Sulfide              | 1.566         | 1.565             | 1.570             | 1.552  | 1.554             | 1.608                | 1.567 | 1.566            |
| Dimethyl Sulfone              | 4.375         | 4.398             | 4.499             | 4.286  | 4.432             | 4.716                | 4.429 | 4.429            |
| Ethanol                       | 1.639         | 1.638             | 1.658             | 1.613  | 1.690             | 1.609                | 1.640 | 1.560            |
| Fluorobenzene                 | 1.340         | 1.376             | 1.464             | 1.376  | 1.600             | 1.576                | 1.428 | 1.427            |
| Furan                         | 0.508         | 0.519             | 0.565             | 0.517  | 0.660             | 0.651                | 0.552 | 0.554            |
| H <sub>2</sub> O              | 1.942         | 1.940             | 1.947             | 1.925  | 1.855             | 1.856                | 1.936 | 1.936            |
| H <sub>2</sub> S              | 1.123         | 1.110             | 1.088             | 1.110  | 0.978             | 0.992                | 1.121 | 1.121            |
| Imidazole                     | 3.813         | 3.810             | 3.811             | 3.746  | 3.800             | 3.784                | 3.810 | 3.810            |
| Isobutene                     | 0.525         | 0.510             | 0.483             | 0.506  | 0.503             | 0.505                | 0.473 | 0.473            |
| Methanol                      | 1.655         | 1.655             | 1.673             | 1.635  | 1.700             | 1.696                | 1.654 | 1.654            |
| Methyl Acetate                | 1.735         | 1.736             | 1.741             | 1.695  | 1.720             | 1.802                | 1.691 | 1.691            |
| Methyl Formate                | 1.848         | 1.846             | 1.847             | 1.824  | 1.770             | 1.821                | 1.800 | 1.742            |
| NH <sub>3</sub>               | 1.640         | 1.633             | 1.630             | 1.614  | 1.472             | 1.518                | 1.622 | 1.622            |
| N-Methylacetamide             | 3.676         | 3.683             | 3.716             | 3.626  | 3.710             | 3.856                | 3.658 | 3.652            |
| NO                            | 0.249         | 0.218             | 0.148             | 0.292  | 0.159             | 0.214                | 0.196 | 0.197            |
| Pentene                       | 0.351         | 0.344             | 0.332             | 0.348  | 0.500             | 0.383                | 0.323 | 0.341            |
| PH <sub>3</sub>               | 0.669         | 0.661             | 0.644             | 0.672  | 0.574             | 1.279                | 0.676 | 0.676            |
| Phenol                        | 1.293         | 1.290             | 1.294             | 1.274  | 1.224             | 0.632                | 1.284 | 1.285            |
| Pyrazole                      | 2.322         | 2.320             | 2.322             | 2.268  | 2.200             | 2.305                | 2.278 | 2.277            |
| Pyridine                      | 2.235         | 2.226             | 2.225             | 2.190  | 2.215             | 2.278                | 2.234 | 2.235            |
| Pyrrole                       | 1.977         | 1.976             | 1.963             | 1.960  | 1.740             | 1.859                | 1.961 | 1.960            |
| SO                            | 1.730         | 1.713             | 1.747             | 1.491  | 1.550             | 1.630                | 1.735 | 1.735            |
| SO <sub>2</sub>               | 1.749         | 1.754             | 1.784             | 1.473  | 1.633             | 1.780                | 1.639 | 1.638            |
| Thiophene                     | 0.415         | 0.442             | 0.499             | 0.419  | 0.550             | 0.514                | 0.403 | 0.405            |
| Toluene                       | 0.355         | 0.346             | 0.333             | 0.344  | 0.375             | 0.377                | 0.335 | 0.335            |
| Trimethylamine                | 0.610         | 0.612             | 0.636             | 0.535  | 0.612             | 0.705                | 0.588 | 0.588            |
| MAE                           | 0.096         | 0.088             | 0.079             | 0.113  | –                 | 0.079                | 0.093 | 0.098            |
| RSMD                          | 0.149         | 0.142             | 0.129             | 0.129  | –                 | 0.133                | 0.150 | 0.168            |

<sup>a</sup>Results taken from Ref. 15

## REFERENCES

- <sup>1</sup>A. Marie and P.-F. Loos, J. Chem. Theory Comput. **19**, 3943 (2023).  
<sup>2</sup>F. A. Evangelista, J. Chem. Phys. **141**, 054109 (2014).  
<sup>3</sup>M. Kállay, J. Chem. Phys. **141**, 244113 (2014).  
<sup>4</sup>D. Mester, P. R. Nagy, and M. Kállay, J. Chem. Phys. **146**, 194102 (2017).  
<sup>5</sup>D. E. Bernholdt and R. J. Harrison, Chem. Phys. Lett. **250**, 477 (1996).  
<sup>6</sup>R. Bauernschmitt, M. Häser, O. Treutler, and R. Ahlrichs, Chem. Phys. Lett. **264**, 573 (1997).  
<sup>7</sup>J. Tölle, N. Niemeyer, and J. Neugebauer, J. Chem. Theory Comput. **20**, 2022 (2024).  
<sup>8</sup>F. Weigend, A. Köhn, and C. Hättig, J. Chem. Phys. **116**, 3175 (2002).  
<sup>9</sup>T. H. Dunning, J. Chem. Phys. **90**, 1007 (1989).  
<sup>10</sup>R. A. Kendall, T. H. Dunning, and R. J. Harrison, J. Chem. Phys. **96**, 6796 (1992).  
<sup>11</sup>B. P. Prascher, D. E. Woon, K. A. Peterson, T. H. Dunning, and A. K. Wilson, Theor. Chem. Acc. **128**, 69 (2011).  
<sup>12</sup>D. E. Woon and T. H. Dunning, J. Chem. Phys. **100**, 2975 (1994).  
<sup>13</sup>J. P. Perdew, K. Burke, and M. Ernzerhof, Phys. Rev. Lett. **77**, 3865 (1996).  
<sup>14</sup>J. P. Perdew, M. Ernzerhof, and K. Burke, J. Chem. Phys. **105**, 9982 (1996).  
<sup>15</sup>A. L. Hickey and C. N. Rowley, J. Phys. Chem. A **118**, 3678 (2014).
